# Supplementary material for: High-throughput computation of electric polarization in solids via Berry flux diagonalization
Source: arXiv:2511.18586 source file (2025-11-23)
Supplement: Supplementary file 1 [file SI.pdf]

# Supplementary Information

Abigail N. Poteshman* Francesco Ricci† Jeffrey B. Neaton‡

## Contents

1 **Input cell parameters for Quantum ESPRESSO** **2**

2 **Manual branch tracing for interpolation-based Berry phase polarization calculations with Quantum ESPRESSO** **4**

3 **Convergence studies with respect to number of $k$-points for Quantum ESPRESSO** **7**

4 **DFT+U calculations for $BiFeO_3$ for Quantum ESPRESSO** **8**

5 **Parallel results for exploring translation and interpolation heuristics in Quantum ESPRESSO** **9**

6 **High-throughput calculation results in VASP** **12**

*Committee on Computational and Applied Mathematics, University of Chicago, Chicago, IL 60637, USA; Materials Science Division, Argonne National Laboratory, Lemont, IL, 60439, USA

†Materials Sciences Division, Lawrence Berkeley National Laboratory, Berkeley, CA 94720, USA; Department of Physics, University of California, Berkeley, CA 94720, USA; Institute of Condensed Matter and Nanosciences (IMCN), Université catholique de Louvain (UCLouvain), Louvain-la-Neuve, Belgium; Matgenix SRL, A6K Advanced Engineering Centre, Charleroi, Belgium

‡Materials Sciences Division, Lawrence Berkeley National Laboratory, Berkeley, CA 94720, USA; Department of Physics, University of California, Berkeley, CA 94720, USA; Kavli Energy NanoSciences Institute at Berkeley, Berkeley, CA 94720, USA.

# 1 Input cell parameters for Quantum ESPRESSO

The structure parameters (and Materials Project (MP) id's) of the polar and nonpolar cells we used as input for the QUANTUM ESPRESSO calculations are reported in Tables 1 & 2. When possible, we used the same structures that were used in the calculations performed in [1] and [2], which are available through the Materials Project [3].

For $BiFeO_3$, we follow the procedure from [2] and obtain the polar structure for the antiferromagnetic configuration by starting from the ferromagnetic structures and space group reported in the Materials Project (mp-24932). This structure was relaxed in VASP with PBE according to the criterion reported in [1]. Then, we imposed an antiferromagnetic configuration and re-relaxed the structure with the correct antiferromagnetic configuration, and these cell parameters are reported in Table 1. For the nonpolar cell, we use a nonpolar cell generated from the polar cell using PSEUDO, and then relaxed the nonpolar structure from PSUEDO, and these cell parameters are reported in Table 2.

| material | polar cell source | polar (a, b, c) (Å) | polar $(\alpha, \beta, \gamma)$ (°) |
|---|---|---|---|
| $BaTiO_3$ | mp-5986 | (4.002, 4.002, 4.216) | (90.0, 90.0, 90.0) |
| $KNbO_3$ | mp-4342 | (4.029, 4.029, 4.219) | (90.0, 90.0, 90.0) |
| $PbTiO_3$ | mp-20459 | (3.872, 3.872, 4.585) | (90.0, 90.0, 90.0) |
| $LiNbO_3$ | mp-3731* | (5.223, 5.223, 14.129) | (90.0, 90.0, 120.0) |
| $Bi_2MoO_6$ | mp-25708* | (5.600, 16.669, 5.625) | (90.0, 90.0, 90.0) |
| $CrO_3$ | mvc-13134* | (5.001, 5.259, 7.129) | (90.0, 89.9, 90.0) |
| $BiFeO_3$ | [2]** | (5.686, 5.686, 5.686) | (59.2, 59.2, 59.2) |

**Table 1:** Polar input cell information and corresponding sources. *The cell parameters for mp-3731 have been updated since the publication of [1], and we report and use the same cell parameters as in [1] to maintain consistency in comparisons between effective polarization values. **$BiFeO_3$ from [2], and see SI Sec. 1 for how the structure was generated.

| material | nonpolar cell source | nonpolar (a, b, c) (Å) | nonpolar $(\alpha, \beta, \gamma)$ (°) |
|---|---|---|---|
| $BaTiO_3$ | mp-2998 | (4.036, 4.036, 4.036) | (90.0, 90.0, 90.0) |
| $KNbO_3$ | mp-935811 | (4.057, 4.057, 4.057) | (90.0, 90.0, 90.0) |
| $PbTiO_3$ | mp-19845 | (3.970, 3.970, 3.970) | (90.0, 90.0, 90.0) |
| $LiNbO_3$ | mp-552588* | (5.269, 5.269, 13.903) | (90.0, 90.0, 120.0) |
| $Bi_2MoO_6$ | mp-567075* | (5.424, 16.949, 5.402) | (90.0, 90.0, 90.0) |
| $CrO_3$ | mp-779986* | (5.852, 4.570, 9.571) | (90.0, 90.0, 90.0) |
| $BiFeO_3$ | [2]** | (5.537, 5.37, 5.537) | (61.2, 61.2, 61.2) |

**Table 2:** Nonpolar input cell information and corresponding sources. *The cell parameters for have been updated since the publication of [1], and we report and use the same cell parameters as in [1] to maintain consistency in comparisons between effective polarization values. **$BiFeO_3$ from [2], and see SI Sec. 1 for how the structure was generated.

## 2 Manual branch tracing for interpolation-based Berry phase polarization calculations with Quantum ESPRESSO

We benchmark the Berry flux diagonalization method for computing effective polarization in Quantum ESPRESSO against the conventional approach, which constructs polarization paths via linear interpolation between polar and nonpolar reference structures. In Quantum ESPRESSO, all polarization branches were manually traced to obtain effective polarization values, including the standard ferroelectric set ($KNbO_3$, $BaTiO_3$, $PbTiO_3$, and $LiNbO_3$), shown in SI Figure 1, as well as materials for which the automated workflow of [1] fails ($Bi_2MoO_6$, $CrO_3$, and $BiFeO_3$), shown in SI Figure 2.

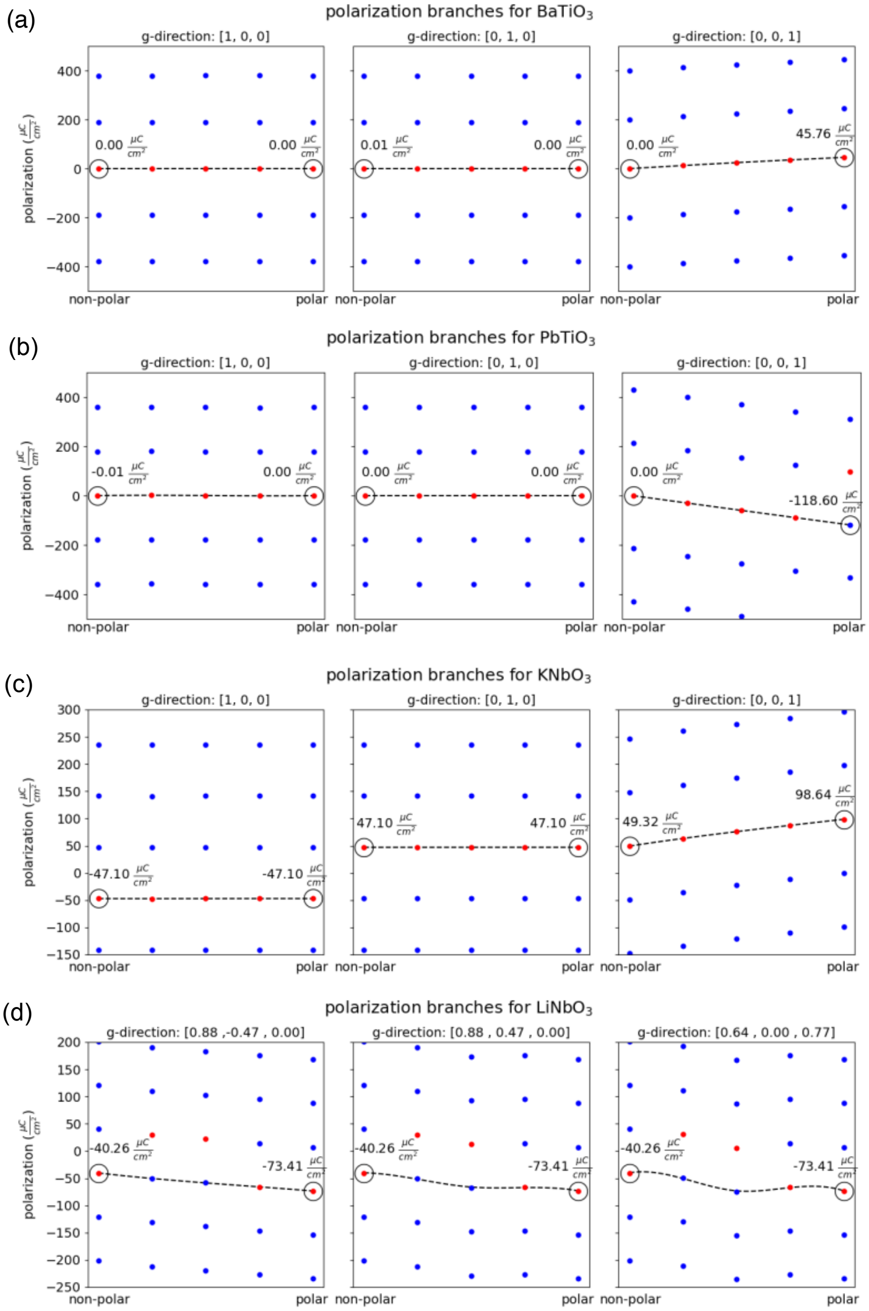


**Figure 1:** Polarization branches for (a) $BaTiO_3$, (b) $PbTiO_3$, (c) $KNbO_3$, and (d) $LiNbO_3$ calculated using the "lberry" tag in QUANTUM ESPRESSO. Polarization values output from QUANTUM ESPRESSO are in red, the polarization branches calculated using the polarization quanta are in blue, the values used for the effective polarization are circled and labeled, and the dashed line is to guide the eye along a proper branch of the polarization.

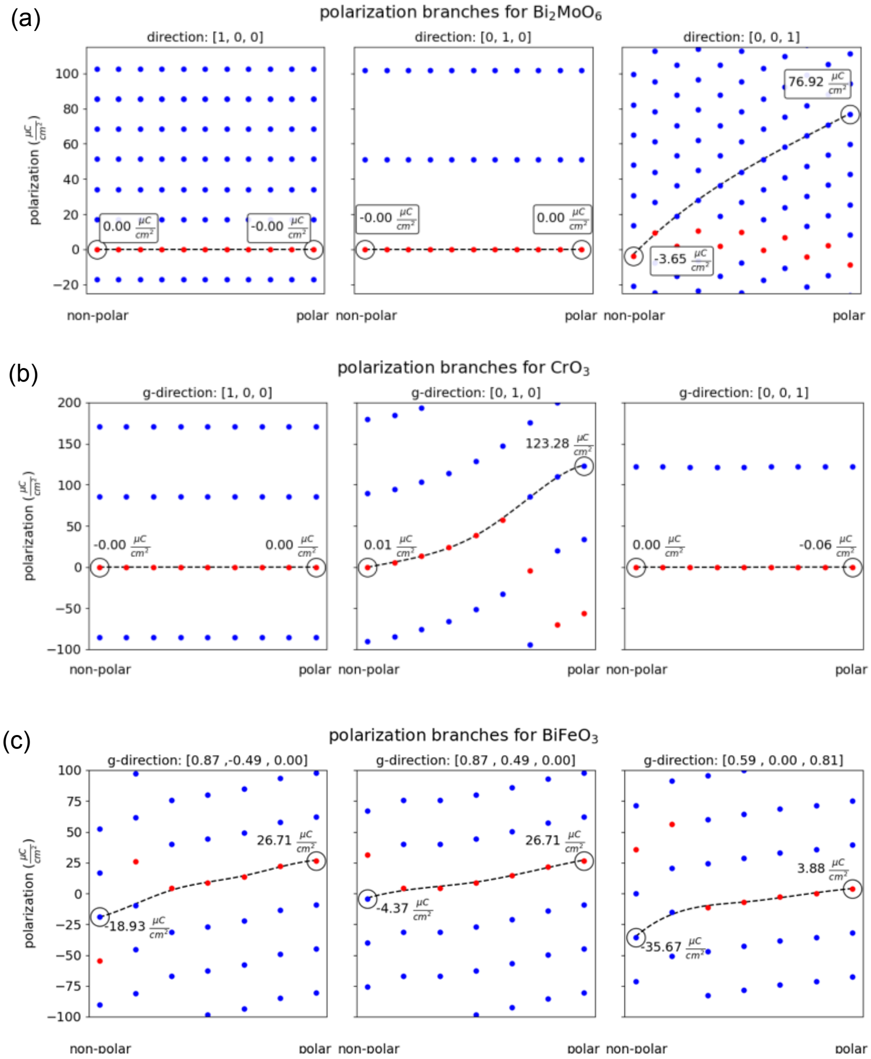


**Figure 2:** Polarization branches for (a) $Bi_2MoO_6$*, (b) $CrO_3^{\dagger}$, and (c) $BiFeO_3$ calculated using the "lberry" tag in QUANTUM ESPRESSO. Polarization values output from QUANTUM ESPRESSO are in red, the polarization branches calculated using the polarization quanta are in blue, the values used for the effective polarization are circled and labeled, and the dashed line is to guide the eye along a proper branch of the polarization. *We used a $9 \times 9 \times 9$ $k$-points in the scf calculation and $18 \times 9 \times 9$ $k$-points in the [1, 0, 0] $g$-direction (and likewise for the [0, 1, 0] and [0, 0, 1] $g$-directions) with 15 strings per $k$-point for $Bi_2MoO_6$. †We used $9 \times 9 \times 9$ $k$-points in the scf calculation and $18 \times 27 \times 18$ $k$-points with 15 strings per $k$-point for the [0, 1, 0] $g$-direction of $CrO_3$.

# 3 Convergence studies with respect to number of $k$-points for Quantum ESPRESSO

For the standard ferroelectrics, $BaTiO_3$, $KNbO_3$, and $PbTiO_3$, we see that the values of effective polarization are converged within 0.5 $^{\mu C}/_{cm^2}$, the minimal singular values from all SVD decompositions of the overlap matrices are converged within 0.02 and the maximum eigenvalues are converged within and for $k$-point meshes ranging from 125 $k$-points ($5 \times 5 \times 5$) to 1331 $k$-points ($11 \times 11 \times 11$) (see Fig. 3). While the maximum eigenvalues decrease with additional $k$-points, even for sparse $k$-point grids, the maximum eigenvalues remains below the threshold value of $\pi$ to ensure that effective polarization is computed along the proper branch.

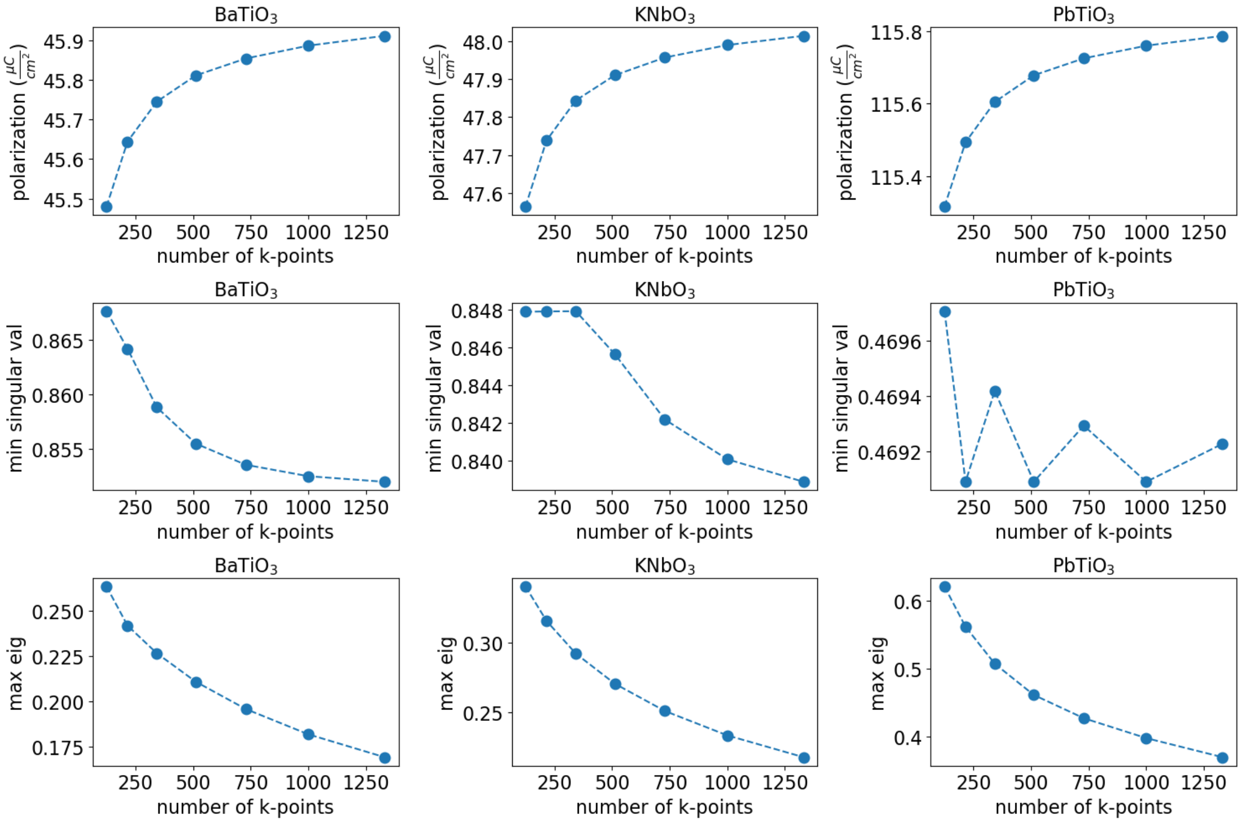


**Figure 3:** Convergence of effective polarization values computed using the Berry flux diagonalization method with respect to $k$-point grid. All calculations were carried out using the translation between polar structure and nonpolar reference structure that minimized the maximal atomic displacement, and we used $k$-grids ranging from $5 \times 5 \times 5$ to $11 \times 11 \times 11$, with $k$-grids increasing by an integer along each direction.

# 4 DFT+U calculations for $BiFeO_3$ for Quantum ESPRESSO

| $U$ (ev) | Effective polarization using BFD ($\frac{\mu C}{cm^2}$) |
|---|---|
| 0 | 94.5 |
| 3 | 93.3 |
| 5 | 92.7 |

**Table 3:** Dependence of $BiFeO_3$ on effective $U$ values

Due to the multiferroic nature of $BiFeO_3$ [4], we used DFT+U to calculate the wavefunctions in Quantum ESPRESSO, and the dependence of the effective polarization value on $U$ is shown in Table 3. In [4], they use a $U_{eff} = 2$ eV with LSDA+U and report an effective polarization value of 95.05 $\mu C/cm^2$.

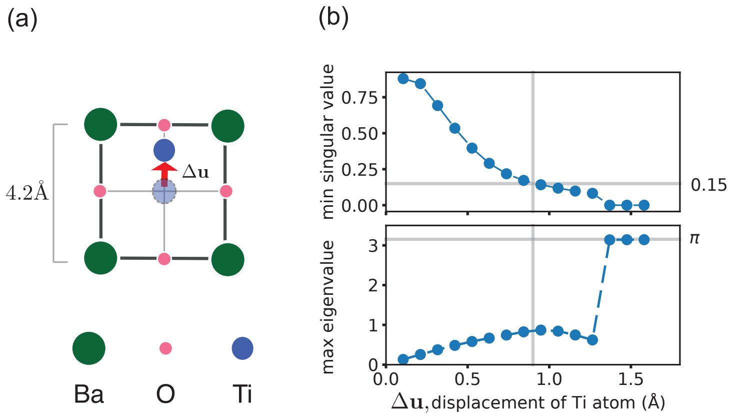


**Figure 4:** (a) Schematic of cubic perovskite $BaTiO_3$ system with fixed Ba and O atoms and a Ti atom that is artificially displaced along the [001] direction (red arrow). The displacement of the Ti atom, $\mathbf{\Delta u}$ , is the difference between its artificial position and its centrosymmetric position. (b) Minimal singular values of the overlap matrices $M^{\langle i,i+1\rangle}$ and maximal eigenvalues of the unitary evolution matrices $U_{\mathcal{P}}$ corresponding to the effective polarization calculated using Berry flux diagonalization for the $BaTiO_3$ with the artificially displaced Ti atom.

# 5 Parallel results for exploring translation and interpolation heuristics in Quantum ESPRESSO

We perform the same set of experiments in Quantum ESPRESSO as described in Sec. III.B of the main text and report the results here.

In SI Fig. 4, we reproduce the behavior observed in VASP for the artificial $BaTiO_3$ test system (Sec. III.B.1). Specifically, increasing the ionic displacement of the central Ti atom leads to a decrease in the minimal singular value of the overlap matrices and an increase in the maximal eigenvalues.

In SI Fig. 5, applying rigid translations to $BaTiO_3$, $KNbO_3$, $PbTiO_3$, and $LiNbO_3$ using Quantum ESPRESSO yields trends consistent with those obtained with VASP (Sec. III.B.2, Fig. 4). For $BaTiO_3$, $KNbO_3$, and $PbTiO_3$, numerical stability is maximized for translations that minimize the maximal atomic displacement, and the effective polarization computed via Berry flux diagonalization agrees with the values obtained from manual interpolation-based calculations in Quantum ESPRESSO (see SI Sec. 2 for the branch calculations). For $LiNbO_3$, however, the translation that minimizes the maximal atomic displacement results in poor numerical stability and inaccurate effective polarization values, indicating the need to use interpolated structures to compute effective polarization along the proper branch.

SI Fig. 6 shows that increasing the number of interpolated structures improves stability for $CrO_3$ and $LiNbO_3$, increasing minimal singular values and reducing maximal eigenvalues. For $LiNbO_3$, sufficient interpolations are essential for accurate effective polarization, whereas $CrO_3$ converges even with poor stability. These results confirm that the heuristics we develop are conservative: they flag potentially inaccurate effective polarization values but are not strictly required to obtain correct results in all cases.

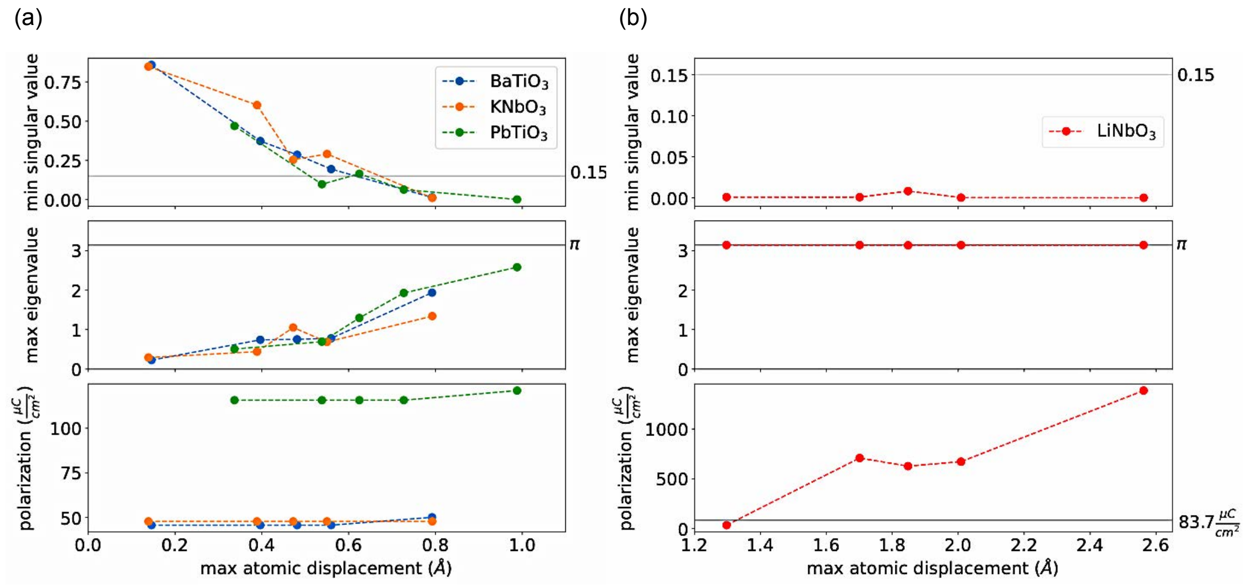


**Figure 5:** Minimal singular values (top), maximal eigenvalues (middle), and effective polarization (bottom) computed from overlap matrices for standard ferroelectrics under different translations of the nonpolar structure relative to the polar structure for (a) $BaTiO_3$, $KNbO_3$, and $PbTiO_3$, and (b) $LiNbO_3$. The translations that minimize the maximal atomic displacement ensure sufficient overlap between wavefunctions at each $k$-point, with minimal singular values remaining above the threshold of 0.15 and maximal eigenvalues below $\pi$. These conditions guarantee proper branch alignment and accurate effective polarization calculations. For $LiNbO_3$, even the translation minimizing maximal atomic displacement results in insufficient overlap, with singular values approaching zero and eigenvalues near $\pi$, leading to improper resolution of polarization branches and inaccurate values of effective polarization.

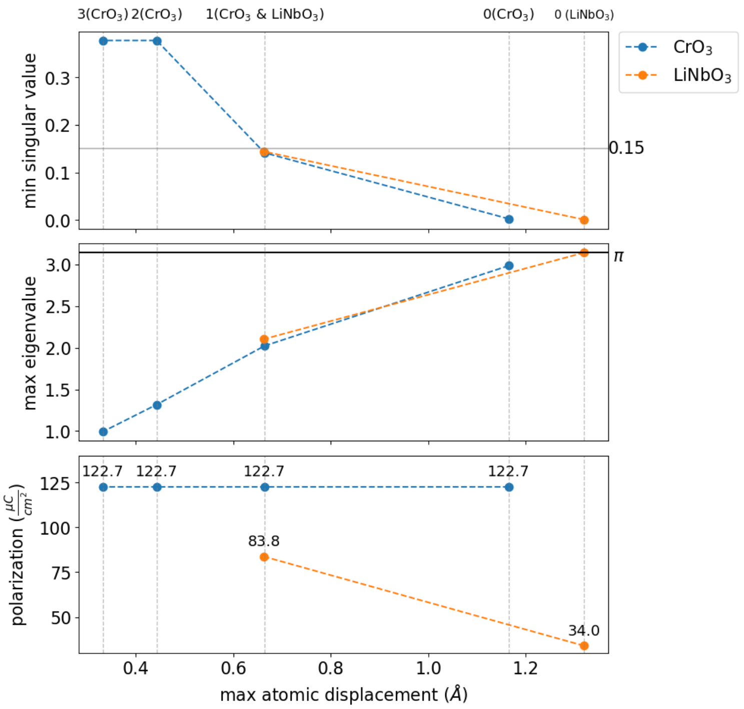


**Figure 6:** Calculated minimum singular values (top), maximal eigenvalues (middle) and effective polarization (bottom) as functions of the maximum atomic displacement for $CrO_3$, $LiNbO_3$, and computed from different numbers of interpolated structures, where the number of interpolations is labeled on the top $x$-axis. For points corresponding to calculations with more than one interpolation, the numbers plotted are the maxima of the maximum atomic displacements across the sets of adjacent interpolated structures used in the intermediate steps of the computation, and likewise for the maxima of the maximum eigenvalues and minima of the minium singular values.

# 6 High-throughput calculation results in VASP

We present in Table 4 the effective polarization values computed using our automated implementation of Berry flux diagonalization with the reference effective polarization values computed with the same polar and nonpolar relaxed structures using the interpolation-based approach in [2]. All calculations were done in VASP v6.4.2 with the default settings for static calculations provided by the Materials Project [3] and ATOMATE2 [5], with the that exception we use PBE v.54 to maintain consistency with the polarization values computed in [2].

| material | mp-ID | FE DB effective polarization ($\mu C/cm^2$) | BFD effective polarization ($\mu C/cm^2$) | # interps (BFD) | min. singular value | max. eigenvalue |
|---|---|---|---|---|---|---|
| $BeO$ | mp-2542 | 121.5 | 121.5 | 1 | 0.85 | 0.21 |
| $Y_3TlF_{10}$ | mp-1207844 | 55.7 | 55.6 | 4 | 0.64 | 0.33 |
| $AlHO_2$ | mp-625054 | 24.1 | 24.1 | 0 | 0.78 | 0.19 |
| $BaNa(B_3O_5)_3$ | mp-17864 | 11.7 | 11.7 | 1 | 0.39 | 0.23 |
| $H_2O$ | mp-697111 | 25.8 | 25.9 | 1 | 0.96 | 0.05 |
| $AsF_3$ | mp-28027 | 69.0 | 69.0 | 1 | 0.65 | 0.31 |
| $Li_2Si_2O_5$ | mp-4117 | 84.1 | 84.1 | 1 | 0.81 | 0.16 |
| $Li_2SiO_3$ | mp-5012 | 77.9 | 77.9 | 1 | 0.86 | 0.16 |
| $CsSO_3$ | mp-561681 | 10.9 | 10.9 | 2 | 0.73 | 0.14 |
| $Na_5B_2P_3O_{13}$ | mp-557836 | 42.7 | 42.7 | 4 | 0.35 | 0.26 |
| $Ga_3Pb_5F_{19}$ | mp-556117 | 16.6 | 16.5 | 2 | 0.71 | 0.24 |
| $LiSiNO$ | mp-6015 | 110.3 | 110.2 | 1 | 0.87 | 0.22 |
| $Zn(PO_3)_2$ | mp-558930 | 26.4 | 26.4 | 4 | 0.37 | 0.15 |
| $ScHO_2$ | mp-625150 | 22.1 | 22.2 | 0 | 0.78 | 0.19 |
| $Na_3HfF_7$ | mp-34579 | 26.0 | 26.0 | 2 | 0.51 | 0.16 |
| $KLiSi_2O_5$ | mp-558102 | 69.5 | 69.5 | 1 | 0.64 | 0.30 |
| $BaZnF_4$ | mp-3881 | 12.2 | 12.2 | 1 | 0.67 | 0.16 |
| $Sr_7Y_6OF_{30}$ | mp-1218554 | 10.3 | 10.3 | 2 | 0.79 | 0.22 |
| $K_2Si_2O_5$ | mp-29825 | 24.2 | 24.2 | 3 | 0.79 | 0.23 |
| $NaSb_3F_{10}$ | mp-27573 | 50.4 | 50.4 | 3 | 0.72 | 0.14 |
| $RbH_3O_2$ | mp-28264 | 28.1 | 28.1 | 0 | 0.59 | 0.45 |
| $LiI$ | mp-570935 | 21.9 | 21.9 | 1 | 0.82 | 0.23 |
| $CsAsF_4$ | mp-5707 | 21.6 | 21.6 | 1 | 0.80 | 0.30 |
| $NaHSeO_4$ | mp-1220802 | 14.9 | 14.9 | 0 | 0.80 | 0.22 |
| $NaAlO_2$ | mp-9212 | 77.9 | 77.9 | 1 | 0.61 | 0.21 |
| $Li_2GeO_3$ | mp-15349 | 75.8 | 75.8 | 1 | 0.64 | 0.17 |
| $TePb_3Cl_4O_3$ | mp-1196950 | 32.8 | 32.7 | 3 | 0.77 | 0.48 |
| $TaTlWO_6$ | mp-1217830 | 14.1 | 14.0 | 0 | 0.55 | 0.39 |
| $Al_2PbO_4$ | mp-21892 | 96.8 | 96.8 | 1 | 0.59 | 0.23 |
| $Ga_2PbO_4$ | mp-20496 | 99.3 | 99.2 | 1 | 0.42 | 0.26 |
| $LiTaO_3$ | mp-3666 | 57.8 | 57.6 | 1 | 0.84 | 0.19 |
| $Rb_5Nb_3OF_{18}$ | mp-540995 | 11.2 | 11.0 | 2 | 0.70 | 0.19 |

| material | mp-ID | FE DB effective polarization ($^{\mu C}/_{cm^2}$) | BFD effective polarization ($^{\mu C}/_{cm^2}$) | # interps (BFD) | min. singular value | max. eigenvalue |
|---|---|---|---|---|---|---|
| $KNaGeO_3$ | mp-558085 | 39.7 | 39.7 | 0 | 0.14 | 0.35 |
| $Al_2CdBr_8$ | mp-1214910 | 32.4 | 32.4 | 5 | 0.57 | 0.17 |
| $Cd(GaCl_4)_2$ | mp-1213982 | 36.2 | 36.2 | 3 | 0.26 | 0.17 |
| $Ta_2Pb_2O_7$ | mp-755663 | 40.6 | 40.3 | 0 | 0.61 | 0.38 |
| $KNbWO_6$ | mp-1223396 | 25.5 | 25.2 | 1 | 0.87 | 0.20 |
| $Li_2MgGeO_4$ | mp-1210797 | 86.6 | 86.6 | 1 | 0.50 | 0.18 |
| $Rb_2Cd(IBr)_2$ | mp-1103709 | 20.4 | 20.4 | 3 | 0.53 | 0.22 |
| $KNbSi_2O_7$ | mp-560407 | 22.5 | 22.0 | 0 | 0.82 | 0.18 |
| $Ca_4YB_3O_{10}$ | mp-1214020 | 28.1 | 28.0 | 3 | 0.72 | 0.18 |
| $TlSbWO_6$ | mp-1216623 | 11.2 | 11.2 | 0 | 0.70 | 0.37 |
| $Ca_2Nb_2O_7$ | mp-13979 | 22.6 | 22.1 | 1 | 0.75 | 0.28 |
| $ZnBi_6P_2O_{15}$ | mp-645375 | 35.1 | 35.0 | 1 | 0.50 | 0.26 |
| $Bi_4Br_2O_5$ | mp-23544 | 24.6 | 24.5 | 1 | 0.59 | 0.19 |
| $BaTi(IO_3)_6$ | mp-1227524 | 10.4 | 10.4 | 2 | 0.77 | 0.24 |
| $Li_3AsO_4$ | mp-9197 | 89.6 | 89.6 | 1 | 0.84 | 0.23 |
| $BaCa(GaO_2)_4$ | mp-561446 | 85.5 | 85.5 | 1 | 0.43 | 0.22 |
| $CaTa_2Bi_2O_9$ | mp-556697 | 40.9 | 40.9 | 1 | 0.59 | 0.21 |
| $Ba_5Re_3NO_{18}$ | mp-555095 | 23.3 | 23.4 | 3 | 0.80 | 0.17 |
| $KYSiS_4$ | mp-867328 | 10.1 | 10.1 | 1 | 0.84 | 0.20 |
| $AgIO_3$ | mp-27384 | 19.1 | 19.1 | 1 | 0.61 | 0.22 |
| $TiBi_2O_5$ | mp-752676 | 35.1 | 35.1 | 1 | 0.72 | 0.19 |
| $BaAl_4S_7$ | mp-8258 | 45.2 | 45.2 | 1 | 0.82 | 0.30 |
| $NaNbSe_2O_7$ | mp-1190450 | 14.0 | 13.6 | 0 | 0.65 | 0.17 |
| $RbSbMoO_6$ | mp-1219606 | 28.5 | 28.2 | 0 | 0.80 | 0.30 |
| $NaLi_2AsO_4$ | mp-9066 | 81.0 | 81.0 | 1 | 0.68 | 0.22 |
| $Rb_2Mo_3SeO_{12}$ | mp-1198721 | 68.4 | 67.8 | 3 | 0.77 | 0.36 |
| $TiI_2O_7$ | mp-1205304 | 12.9 | 12.9 | 0 | 0.87 | 0.17 |
| $NaGaO_2$ | mp-3338 | 73.3 | 73.3 | 1 | 0.45 | 0.20 |
| $SrMgH_4$ | mp-643009 | 18.2 | 18.2 | 1 | 0.74 | 0.21 |
| $CsGeCl_3$ | mp-22988 | 22.5 | 22.4 | 0 | 0.31 | 0.63 |
| $Na_3VO_4$ | mp-755436 | 69.0 | 68.9 | 1 | 0.57 | 0.71 |
| $SeOF_2$ | mp-27367 | 85.7 | 85.6 | 2 | 0.75 | 0.32 |
| $Na_3PSO_3$ | mp-542136 | 41.4 | 41.5 | 1 | 0.85 | 0.27 |
| $Li_3VO_4$ | mp-19219 | 86.6 | 86.7 | 1 | 0.76 | 0.45 |
| $LiAlS_2$ | mp-1106183 | 60.3 | 60.3 | 1 | 0.83 | 0.32 |
| $GaClO$ | mp-1212662 | 50.0 | 49.9 | 1 | 0.48 | 0.16 |
| $Mg_2PN_3$ | mp-3933 | 91.5 | 91.4 | 1 | 0.85 | 0.34 |
| $BrF_5$ | mp-27987 | 25.3 | 25.3 | 1 | 0.79 | 0.31 |
| $CsGeBr_3$ | mp-1068340 | 20.0 | 19.9 | 0 | 0.38 | 0.69 |
| $Nb_3Al(PO_4)_6$ | mp-1220763 | 88.3 | 88.2 | 3 | 0.70 | 0.25 |
| $TiSb(PO_4)_3$ | mp-1239394 | 83.2 | 83.2 | 3 | 0.72 | 0.24 |

| material | mp-ID | FE DB effective polarization ($\mu C/cm^2$) | BFD effective polarization ($\mu C/cm^2$) | # interps (BFD) | min. singular value | max. eigenvalue |
|---|---|---|---|---|---|---|
| $Sr_2Nb_2O_7$ | mp-3870 | 38.9 | 38.1 | 1 | 0.64 | 0.19 |
| $NbTlTeO_6$ | mp-1220473 | 25.2 | 24.7 | 0 | 0.55 | 0.30 |
| $Sc_2TiO_5$ | mp-753401 | 35.3 | 35.2 | 2 | 0.77 | 0.16 |
| $KYGeS_4$ | mp-867334 | 11.0 | 10.9 | 1 | 0.81 | 0.23 |
| $Ga_2S_3$ | mp-539 | 60.9 | 60.7 | 2 | 0.25 | 0.41 |
| $Al_2Se_3$ | mp-11674 | 54.7 | 54.6 | 2 | 0.76 | 0.41 |
| $Ti_3P_6WO_{24}$ | mp-775198 | 87.8 | 87.8 | 3 | 0.70 | 0.24 |
| $Tl_3AsO_4$ | mp-15573 | 43.9 | 43.9 | 1 | 0.77 | 0.23 |
| $TiNb(PO_4)_3$ | mp-1216943 | 87.0 | 87.0 | 3 | 0.69 | 0.25 |
| $TaTi(PO_4)_3$ | mp-1244815 | 86.5 | 86.5 | 3 | 0.69 | 0.25 |
| $TlSnPS_4$ | mp-6057 | 15.1 | 15.1 | 1 | 0.74 | 0.20 |
| $BrF_3$ | mp-23297 | 30.7 | 30.7 | 2 | 0.77 | 0.15 |
| $PSeCl_9$ | mp-662547 | 13.0 | 13.0 | 2 | 0.80 | 0.34 |
| $BiIO_4$ | mp-1191266 | 77.7 | 77.6 | 1 | 0.73 | 0.43 |
| $Li_7BiO_6$ | mp-38487 | 15.1 | 15.2 | 2 | 0.81 | 0.14 |
| $KLiZn_3O_4$ | mp-1223469 | 58.2 | 58.3 | 3 | 0.38 | 0.44 |
| $SnPS_3$ | mp-13923 | 32.0 | 31.9 | 1 | 0.73 | 0.30 |
| $K_2Sn_2Hg_3S_8$ | mp-18115 | 45.7 | 45.5 | 3 | 0.50 | 0.40 |
| $SrNb_2Bi_2O_9$ | mp-23614 | 57.7 | 57.1 | 1 | 0.68 | 0.30 |
| $BaGa_4S_7$ | mp-4309 | 43.9 | 43.9 | 1 | 0.52 | 0.39 |
| $LiAlSe_2$ | mp-7117 | 54.1 | 54.0 | 1 | 0.74 | 0.45 |
| $RbMoIO_6$ | mp-554787 | 55.6 | 55.5 | 2 | 0.78 | 0.25 |
| $LiGaS_2$ | mp-3647 | 59.8 | 59.7 | 1 | 0.48 | 0.51 |
| $Sr_2SnS_4$ | mp-30294 | 58.0 | 58.0 | 3 | 0.46 | 0.31 |
| $Bi_2WO_6$ | mp-23480 | 53.4 | 53.3 | 1 | 0.78 | 0.24 |
| $MgGeN_2$ | mp-7798 | 123.1 | 122.9 | 1 | 0.52 | 0.34 |
| $LiInS_2$ | mp-1188392 | 54.6 | 54.5 | 1 | 0.68 | 0.41 |
| $ClF_5$ | mp-1213763 | 31.2 | 31.2 | 1 | 0.73 | 0.39 |
| $Bi_{10}(MoO_8)_3$ | mp-558215 | 10.6 | 10.6 | 4 | 0.74 | 0.29 |
| $Li_2Mo_3S_4$ | mp-675779 | 14.4 | 14.4 | 1 | 0.70 | 0.44 |
| $TaZn_2N_3$ | mp-1029387 | 118.9 | 118.9 | 1 | 0.50 | 0.40 |
| $KNa_2CuO_2$ | mp-545359 | 22.8 | 22.9 | 1 | 0.58 | 0.11 |
| $SnPSe_3$ | mp-570370 | 24.7 | 24.6 | 0 | 0.64 | 0.57 |
| $Ga_2Sn_2S_5$ | mp-14280 | 21.4 | 21.5 | 6 | 0.26 | 0.39 |
| $Bi_2TeO_5$ | mp-23334 | 59.6 | 59.5 | 3 | 0.76 | 0.22 |
| $Li_2CdGeO_4$ | mp-7688 | 82.3 | 82.2 | 1 | 0.35 | 0.19 |
| $Ag_2HgSI_2$ | mp-556866 | 11.7 | 11.6 | 1 | 0.73 | 0.24 |
| $RbGeBr_3$ | mp-28558 | 11.2 | 11.1 | 0 | 0.10 | 0.65 |
| $NbZn_2N_3$ | mp-1029422 | 115.8 | 116.0 | 1 | 0.51 | 0.40 |
| $NbTlBr_4O$ | mp-551826 | 17.8 | 17.4 | 0 | 0.78 | 0.37 |
| $GaSeBr_7$ | mp-23376 | 26.4 | 26.2 | 3 | 0.16 | 0.32 |

| material | mp-ID | FE DB effective polarization ($\mu C/cm^2$) | BFD effective polarization ($\mu C/cm^2$) | # interps (BFD) | min. singular value | max. eigenvalue |
|---|---|---|---|---|---|---|
| $Mg_2SbN_3$ | mp-1029378 | 103.1 | 103.0 | 0 | 0.69 | 0.47 |
| CdS | mp-672 | 51.2 | 51.1 | 1 | 0.68 | 0.32 |
| $VZn_2N_3$ | mp-1029262 | 120.9 | 120.8 | 1 | 0.48 | 0.57 |
| $YTl(PSe_3)_2$ | mp-1105136 | 13.5 | 13.5 | 4 | 0.68 | 0.28 |
| $Li_2CdSnS_4$ | mp-1188784 | 55.4 | 55.3 | 1 | 0.61 | 0.52 |
| $LiGaSe_2$ | mp-11582 | 53.9 | 53.7 | 1 | 0.36 | 0.52 |
| $SrTaNO_2$ | mp-1101327 | 42.0 | 41.7 | 0 | 0.69 | 0.46 |
| $TlVTeO_5$ | mp-639714 | 61.4 | 61.4 | 3 | 0.66 | 0.30 |
| $Sr_{14}(SnAs_4)_3$ | mp-1192393 | 20.0 | 20.0 | 2 | 0.69 | 0.46 |
| $Ca_5NbN_5$ | mp-675101 | 39.3 | 39.3 | 4 | 0.70 | 0.20 |
| $TiZnN_2$ | mp-1016108 | 121.1 | 121.0 | 0 | 0.19 | 0.65 |
| $Li_2CdGeS_4$ | mp-1189383 | 58.3 | 58.3 | 1 | 0.30 | 0.51 |
| $CaSnN_2$ | mp-1029633 | 88.1 | 88.0 | 1 | 0.61 | 0.33 |
| $Ag_2GeS_3$ | mp-9900 | 49.3 | 49.3 | 1 | 0.49 | 0.60 |
| $NbBr_2O$ | mp-550070 | 23.4 | 22.7 | 0 | 0.80 | 0.28 |
| $NbI_2O$ | mp-549720 | 17.5 | 16.7 | 0 | 0.64 | 0.32 |
| $NbCl_2O$ | mp-1025567 | 26.9 | 26.1 | 0 | 0.82 | 0.27 |
| $CsGeI_3$ | mp-28377 | 17.6 | 17.7 | 0 | 0.29 | 0.69 |
| $Ba_2In_2O_5$ | mp-20546 | 26.9 | 26.9 | 1 | 0.58 | 0.29 |
| MgTe | mp-1039 | 42.7 | 42.7 | 1 | 0.67 | 0.43 |
| $Li_2ZnGeS_4$ | mp-1210804 | 61.6 | 61.6 | 1 | 0.33 | 0.50 |
| $Mg_2VN_3$ | mp-1029368 | 99.5 | 99.5 | 1 | 0.74 | 0.74 |
| $Li_3SbS_4$ | mp-756316 | 56.6 | 56.5 | 1 | 0.58 | 0.75 |
| $CsIO_3$ | mp-28295 | 73.4 | 73.3 | 1 | 0.67 | 0.96 |
| $Ca_{11}AlSb_9$ | mp-1214215 | 17.6 | 17.5 | 3 | 0.51 | 0.53 |
| $KCu(BiS_2)_2$ | mp-558063 | 14.3 | 14.2 | 1 | 0.50 | 0.20 |
| $LiVN_2$ | mp-1029932 | 124.8 | 124.9 | 1 | 0.56 | 0.94 |
| GeTe | mp-938 | 66.7 | 68.8 | 0 | 0.24 | 0.92 |
| $Ba_2Ge_2Te_5$ | mp-17885 | 11.5 | 11.6 | 4 | 0.25 | 0.40 |
| $Hg(IO_3)_2$ | mp-23407 | 36.6 | 36.4 | 3 | 0.80 | 0.34 |
| $Cd_2GaAgS_4$ | mp-6356 | 55.1 | 55.0 | 1 | 0.35 | 0.46 |
| $Ca_2CdP_2$ | mp-1078908 | 14.7 | 14.8 | 2 | 0.57 | 0.22 |
| $RbHgSbTe_3$ | mp-1219595 | 14.6 | 14.8 | 0 | 0.28 | 0.84 |
| $Ba_2InBiS_5$ | mp-864638 | 28.0 | 28.1 | 2 | 0.33 | 0.34 |
| $ClO_3$ | mp-22869 | 43.0 | 43.0 | 2 | 0.66 | 0.66 |
| $Cs_2Te_3$ | mp-505634 | 28.5 | 29.4 | 1 | 0.19 | 1.08 |
| $Ca_2CdAs_2$ | mp-1095180 | 15.5 | 15.6 | 2 | 0.25 | 0.28 |
| $NaNbS_6$ | mp-1210002 | 15.4 | 15.4 | 3 | 0.46 | 0.40 |
| $K_2Se_3$ | mp-7670 | 40.1 | 40.1 | 1 | 0.47 | 0.74 |
| SrGaSiH | mp-979137 | 39.6 | 39.6 | 1 | 0.55 | 0.34 |
| $Li_5SiP_3$ | mp-685991 | 31.8 | 31.8 | 1 | 0.53 | 0.34 |

| material | mp-ID | FE DB effective polarization ($\mu C/cm^2$) | BFD effective polarization ($\mu C/cm^2$) | # interps (BFD) | min. singular value | max. eigenvalue |
|---|---|---|---|---|---|---|
| SrAlGeH | mp-980057 | 40.0 | 40.1 | 1 | 0.61 | 0.33 |
| $LiAsS_2$ | mp-555874 | 81.9 | 81.9 | 1 | 0.03 | 1.19 |
| $Sr_2CdAs_2$ | mp-867203 | 11.7 | 11.8 | 2 | 0.12 | 0.34 |
| $Cs_2Se_3$ | mp-7449 | 34.0* | 31.3 | 1 | 0.01 | 1.09 |
| $LiB(SO_4)_2$ | mp-1020106 | 57.1* | 57.1 | 4 | 0.74 | 0.33 |
| $Li_3AlSiO_5$ | mp-1020023 | 85.4* | 85.4 | 1 | 0.86 | 0.15 |
| $B_4PbO_7$ | mp-9747 | 118.2* | 118.1 | 1 | 0.58 | 0.41 |
| $Li_3AlGeO_5$ | mp-6765 | 82.6* | 82.7 | 1 | 0.53 | 0.15 |
| $Li_3GaSiO_5$ | mp-16996 | 84.6* | 84.5 | 1 | 0.44 | 0.14 |
| $Li_3GaGeO_5$ | mp-17685 | 81.8* | 81.8 | 1 | 0.54 | 0.16 |
| $Ti(SO_4)_2$ | mp-775149 | 107.6* | 107.6 | 4 | 0.67 | 0.36 |
| $Sb_6S_2O_{15}$ | mp-27229 | 57.3* | 57.2 | 2 | 0.81 | 0.15 |
| $Bi_2MoO_6$ | mp-23064 | 78.0* | 77.4 | 1 | 0.72 | 0.51 |
| $KAu(IO_3)_4$ | mp-557441 | 135.5* | 135.4 | 4 | 0.62 | 1.33 |
| $Ba_2InBiSe_5$ | mp-1105202 | 30.0* | 29.7 | 2 | 0.23 | 2.51 |
| $K_4Ba_2SnAs_4$ | mp-1224063 | 6.1* | 6.1 | 2 | 0.46 | 0.52 |
| $K_4Ba_2SnSb_4$ | mp-1224100 | 7.5* | 8.1 | 2 | 0.00 | 1.66 |
| $K_4Ba_2SnBi_4$ | mp-1224198 | 6.7* | 7.5 ($6.5^\dagger$) | 3 ($9^\dagger$) | 0.10 ($0.19^\dagger$) | 2.18 ($2.76^\dagger$) |
| $Rb_2Se_3$ | mp-7447 | 38.7* | 32.7 ($38.5^\ddagger$) | 1 | 0.00 ($0.40^\ddagger$) | 1.19 ($0.75^\ddagger$) |
| $Ba_2InSbSe_5$ | mp-1189339 | 25.8* | 29.9 ($27.9^\ddagger$) | 2 | 0.12 ($0.19^\ddagger$) | 2.19 ($2.16^\ddagger$) |
| $Ba_2CdAs_2$ | mp-1079666 | 14.6 | 6.1 ($10.1^\ddagger$) | 2 | 0.00 ($0.34^\ddagger$) | 1.21 ($0.47^\ddagger$) |

**Table 4:** The FE DB effective polarization values were computed in [2] using a standard 10 interpolated structures unless denoted with *, which denotes that the reference value for the FE DB effective polarization using the standard interpolation-based approach was computed with 20 interpolated structures. The parenthetical effective polarization, minimum singular, and maximum eigenvalue values denoted with $^\dagger$ correspond to corrected values of polarization computed with Berry flux diagonalization for a higher number of interpolations (also given parenthetically) than heuristic number of interpolations. The parenthetical effective polarization, minimum singular, and maximum eigenvalue values denoted with $^\ddagger$ correspond to corrected values of effective polarization computed with twice the default number of $k$-points for static calculations in ATOMATE2 [5]. In the main text, the values computed with the original heuristics are plotted in Figure 6, but both original and recomputed values are presented here.

# References


[1] Tess E Smidt, Stephanie A Mack, Sebastian E Reyes-Lillo, Anubhav Jain, and Jeffrey B Neaton. An automatically curated first-principles database of ferroelectrics. *Scientific Data*, 7(1):72, 2020.

[2] Francesco Ricci, Sebastian E Reyes-Lillo, Stephanie A Mack, and Jeffrey B Neaton. Candidate ferroelectrics via ab initio high-throughput screening of polar materials. *npj*

*Computational Materials*, 10(1):15, 2024.

[3] Anubhav Jain, Shyue Ping Ong, Geoffroy Hautier, Wei Chen, William Davidson Richards, Stephen Dacek, Shreyas Cholia, Dan Gunter, David Skinner, Gerbrand Ceder, et al. Commentary: The materials project: A materials genome approach to accelerating materials innovation. *APL materials*, 1(1), 2013.

[4] JB Neaton, C Ederer, UV Waghmare, NA Spaldin, and KM Rabe. First-principles study of spontaneous polarization in multiferroic bi fe o 3. *Physical Review B*, 71(1):014113, 2005.

[5] Alex M Ganose, Hrushikesh Sahasrabuddhe, Mark Asta, Kevin Beck, Tathagata Biswas, Alexander Bonkowski, Joana Bustamante, Xin Chen, Yuan Chiang, Daryl C Chrzan, et al. Atomate2: Modular workflows for materials science. *Digital Discovery*, 2025.
